# Supplementary material for: Table-based Fact Verification with Salience-aware Learning
Source: arXiv:2109.04053 source file (2021-09-09)
Supplement: Supplementary file 1 [file a_appendix.tex]

\clearpage

\appendix

\section{Appendices}

\subsection{Statistics of the Dataset}

Statistics of the TabFact dataset are listed in \Cref{table:dataset}.
Each table comes along with 2 to 20 statements, and consists of 14 rows and 5 columns in average.

\begin{table}[h]
\centering
\begin{tabular}{ccc}
\toprule[2pt]
Split & \#Statement & \# Table  \\ \midrule
Train & 92,283 & 13,182 \\
Validation & 12,792 & 1,696 \\
Test & 12,799 & 1,695 \\ \midrule
Simple & 50,244 & 9,189 \\
Complex & 68,031 & 7,392 \\
\bottomrule[2pt]
\end{tabular}
\caption{Basic statistics of the TabFact dataset.}
\label{table:dataset}
\end{table} 

\subsection{More Implementation Details}
% Description of computing infrastructure used 
% Number of parameters in each model
% The average runtime for each model or algorithm 
% Bounds for each hyperparameter
% Number of hyperparameter search trials
% The method of choosing hyperparameter values (e.g., uniform sampling, manual tuning, etc.) and the criterion used to select among them (e.g., accuracy) 
% Summary statistics of the results (e.g., mean, variance, error bars, etc.) 

We implement our system based on Transformers\footnote{https://github.com/huggingface/transformers} and Pytorch\footnote{https://github.com/pytorch/pytorch}.
The default system has about 340M parameters.
It takes about 36 hours to train the default system on two NVIDIA Quadro RTX 8000 GPU. 
\Cref{table:hyperparam} shows the search spaces where hyper-parameter values are selected. 
The best configuration is decided based on validation accuracy.

\begin{table}[h]
\centering
\begin{tabular}{lr}
\toprule[2pt]
% \midrule
Hyper-parameters & Search space \\ \midrule
Batch size & \{ 8, 16, 32 \} \\
Learning rate &  \{ $2e^{-5}, 3e^{-5}, 5e^{-5}$ \} \\
$\alpha$ & \{ 0.1, 0.3, 0.5 \} \\
\bottomrule[2pt]
\end{tabular}
\caption{Hyper-parameter search spaces.}
\label{table:hyperparam}
\end{table}
